# Supplementary material for: EE-Grad: Exploration and Exploitation for Cost-Efficient Mini-Batch SGD
Source: arXiv:1705.07070 source file (2017-05-19)
Supplement: Supplementary file 1 [file EEGrad_supplementary.pdf]

## 261 **A Trace of the Sample Covariance Matrix as a Quadratic Form**

262 **Lemma 1.** *On each round  $t$ , the trace of the sample covariance matrix  $\mathbf{Cov}_t(n)$  can be written as*

$$V_t(n) = \mathbf{s}_{t,n}^T \mathbf{A}_{t,n} \mathbf{s}_{t,n}, \quad n = 1, \dots, N,$$

263 where  $\mathbf{s}_{t,n} = \left( \mathbf{G}_1(\mathbf{w}, n)^T, \dots, \mathbf{G}_{\gamma_t(n)}(\mathbf{w}, n)^T \right)^T$ ,  $\mathbf{A}_{t,n} = (\gamma_t(n) - 1)^{-1} \left( \mathbf{I} - \gamma_t(n)^{-1} \mathbf{E} \right)$ ,  $\mathbf{I} \in \mathbb{R}^{d\gamma_t(n) \times d\gamma_t(n)}$   
 264 is an identity matrix, and  $\mathbf{E} \in \mathbb{R}^{d\gamma_t(n) \times d\gamma_t(n)}$  is a block matrix with  $d \times d$  identity blocks.

265 *Proof.* Note that

$$V_t(n) = \text{Tr}(\mathbf{Cov}_t(n)) = \frac{1}{\gamma_t(n) - 1} \left( \sum_{i=1}^{\gamma_t(n)} \mathbf{G}_i(\mathbf{w}, n)^T \mathbf{G}_i(\mathbf{w}, n) - \gamma_t(n) \mathbf{m}_t(n)^T \mathbf{m}_t(n) \right),$$

266 where

$$\mathbf{m}_t(n)^T \mathbf{m}_t(n) = \frac{1}{\gamma_t(n)^2} \sum_{i=1}^{\gamma_t(n)} \sum_{j=1}^{\gamma_t(n)} \mathbf{G}_i(\mathbf{w}, n)^T \mathbf{G}_j(\mathbf{w}, n) = \frac{1}{\gamma_t(n)^2} \mathbf{s}_{t,n}^T \mathbf{E} \mathbf{s}_{t,n}.$$

267 Noting  $\sum_{i=1}^{\gamma_t(n)} \mathbf{G}_i(\mathbf{w}, n)^T \mathbf{G}_i(\mathbf{w}, n) = \mathbf{s}_{t,n}^T \mathbf{s}_{t,n}$ , we conclude that

$$V_t(n) = \frac{1}{\gamma_t(n) - 1} \left( \mathbf{s}_{t,n}^T \mathbf{s}_{t,n} - \frac{1}{\gamma_t(n)} \mathbf{s}_{t,n}^T \mathbf{E} \mathbf{s}_{t,n} \right) = \mathbf{s}_{t,n}^T \mathbf{A}_{t,n} \mathbf{s}_{t,n}.$$

268 □

## 269 **B Hanson-Wright Inequality**

270 **Lemma 2.** *Let  $\mathbf{W} = [W_1, \dots, W_m]^T \in \mathbb{R}^m$ ,  $m > 1$ , where  $W_i$  are zero-mean sub-Gaussian with a  
 271 parameter  $\sigma^2 > 0$ . Then, given an arbitrary matrix  $\mathbf{A} \in \mathbb{R}^{m \times m}$ , we have, for any  $\varepsilon > 0$ ,*

$$\Pr(\mathbf{W}^T \mathbf{A} \mathbf{W} - \mathbb{E}_{\mathbf{W}}[\mathbf{W}^T \mathbf{A} \mathbf{W}] > \varepsilon) \leq \exp \left( -c \min \left( \frac{\varepsilon^2}{\sigma^4 \|\mathbf{A}\|_F^2}, \frac{\varepsilon}{\sigma^2 \|\mathbf{A}\|} \right) \right),$$

272 where  $\|\mathbf{A}\|_F$  and  $\|\mathbf{A}\|$  are Frobenius and operator norms of  $\mathbf{A}$ , and  $c > 0$  is an absolute constant.

## 273 **C Concentration Result on the Trace of the Sample Covariance Matrices**

274 **Lemma 3.** *Suppose that  $\gamma_t(n) > 1$ . Then the tail probability of  $V_t(n)$  satisfies, for any  $\varepsilon > 0$ ,*

$$\Pr(V_t(n) - \sigma_n^2 S(\mathbf{w}) > \varepsilon) \leq \exp(-(\gamma_t(n) - 1)\phi(\varepsilon)),$$

275 where

$$\phi(\varepsilon) \triangleq \frac{c\varepsilon}{\beta P} \min \left( 1, \frac{\varepsilon/d}{\beta P} \right),$$

276 for  $n = 1, \dots, N$ , where  $c > 0$  is an absolute constant.

277 *Proof.* Note that  $\mathbf{I} - (1/\gamma_t(n))\mathbf{E}$  is a  $d\gamma_t(n) \times d\gamma_t(n)$  block matrix with  $d \times d$  blocks, where the  
 278 diagonal and non-diagonal matrices are given by  $\frac{\gamma_t(n)-1}{\gamma_t(n)}\mathbf{I}$  and  $-\frac{1}{\gamma_t(n)}\mathbf{I}$ , respectively, and  $\|\mathbf{I}\|_F^2 = d$ .  
 279 This implies

$$\begin{aligned} \|\mathbf{A}_{t,n}\|_F^2 &= \frac{1}{(\gamma_t(n) - 1)^2} \left( \gamma_t(n) \left( \frac{\gamma_t(n) - 1}{\gamma_t(n)} \right)^2 \|\mathbf{I}\|_F^2 + (\gamma_t(n) - 1) \gamma_t(n) \frac{1}{\gamma_t(n)^2} \|\mathbf{I}\|_F^2 \right) \\ &= \frac{d}{\gamma_t(n) - 1}. \end{aligned}$$

280 Next suppose that  $\mathbf{v} = (\mathbf{v}_1^T, \dots, \mathbf{v}_{\gamma(n)}^T)^T \in \mathbb{R}^{d\gamma(n)}$  such that  $\mathbf{v}_i \in \mathbb{R}^d$  and  $\|\mathbf{v}\|_2 = 1$ . Then we write

$$\begin{aligned}\|\mathbf{A}_{t,n}\mathbf{v}\|_2^2 &= \frac{1}{(\gamma(n)-1)^2} \left( \|\mathbf{v}\|_2^2 + \frac{1}{\gamma(n)^2} \|\mathbf{E}\mathbf{v}\|_2^2 - \frac{2}{\gamma(n)} \mathbf{v}^T \mathbf{E}\mathbf{v} \right) \\ &= \frac{1}{(\gamma(n)-1)^2} \left( 1 - \frac{1}{\gamma(n)} \left\| \sum_{i=1}^{\gamma(n)} \mathbf{v}_i \right\|_2^2 \right) \leq \frac{1}{(\gamma(n)-1)^2},\end{aligned}$$

281 where equality is achieved by  $\mathbf{v} = (\mathbf{v}_1^T, \dots, \mathbf{v}_{\gamma(n)}^T)^T$  such that  $\mathbf{v}_1 = (\frac{1}{\sqrt{2}}, 0, \dots, 0)$ ,  $\mathbf{v}_2 = -\mathbf{v}_1$ , and  
282  $\mathbf{v}_i = (0, \dots, 0)$  for  $i = 3, \dots, \gamma(n)$ . This yields

$$\|\mathbf{A}_{t,n}\| = \sup_{\|\mathbf{v}\|_2=1} \|\mathbf{A}_{t,n}\mathbf{v}\|_2 = (\gamma(n)-1)^{-1}.$$

283 We finally note that the trace of the sample covariance matrix can be written as

$$\begin{aligned}V_t(n) &= \frac{1}{\gamma(n)-1} \sum_{i=1}^{\gamma(n)} (\mathbf{G}_i(\mathbf{w}, n) - \mathbf{m}_t(n))^T (\mathbf{G}_i(\mathbf{w}, n) - \mathbf{m}_t(n)) \\ &= \frac{1}{\gamma(n)-1} \sum_{i=1}^{\gamma(n)} (\mathbf{Q}_i(n) - \mathbf{q}_t(n))^T (\mathbf{Q}_i(n) - \mathbf{q}_t(n)),\end{aligned}$$

284 where  $\mathbf{Q}_i(n) \triangleq \mathbf{G}_i(\mathbf{w}, n) - \nabla F(\mathbf{w})$  for  $i \in [\gamma(n)]$ , and  $\mathbf{q}_t(n) = (1/\gamma(n)) \sum_{i=1}^{\gamma(n)} \mathbf{Q}_i(n)$ . This implies the  
285 same expression holds for the mean-removed versions of  $\mathbf{G}_i(\mathbf{w}, n)$ s. Hence, we can assume that  
286  $\mathbb{E}_{\mathbf{w}}[\mathbf{G}_i(\mathbf{w}, n)] = 0$ . We apply Lemma 2, provided in the supplementary material, to  $V_t(n)$  by using  
287 Lemma 1 to get, for any  $\varepsilon > 0$ ,

$$\Pr(V_t(n) - \sigma_n^2 S(\mathbf{w}) > \varepsilon) \leq \exp(-(\gamma(n)-1)\phi_n(\varepsilon)),$$

288 where

$$\phi_n(\varepsilon) \triangleq \frac{c\varepsilon}{\sigma_n^2 S(\mathbf{w})} \min\left(1, \frac{\varepsilon/d}{\sigma_n^2 S(\mathbf{w})}\right),$$

289 which is strictly increasing in  $\varepsilon$ , for  $n \in [N]$ , where  $c > 0$  is an absolute constant. Finally, we note  
290  $\phi_n(\varepsilon) \geq \phi(\varepsilon)$ , since we assumed  $\max_{n=1, \dots, N} \sigma_n^2 \leq \beta$ , and  $S(\mathbf{w}) \leq P$ . This concludes the proof.  $\square$

## 291 D Pseudo-Regret Bound

292 **Lemma 4.** *For any  $\alpha > 2$ , the pseudo-regret term in (11) satisfies, for any  $T$ ,*

$$\mathbb{E}_{\mathbf{w}} \left[ \sum_{n=1}^N \Delta_n \gamma_T(n) \right] S(\mathbf{w}) \leq (C_1(\mathbf{w}) \ln(T) + C_2) S(\mathbf{w}),$$

293 where

$$C_1(\mathbf{w}) \triangleq \sum_{n: \Delta_n > 0} \frac{\alpha \Delta_n}{\phi(\Delta_n S(\mathbf{w})/2)}, \quad C_2 \triangleq \left( \sum_{n=1}^N \Delta_n \right) \frac{2(\alpha-1)}{\alpha-2}. \quad (\text{D.1})$$

294 *Proof.* We follow along similar steps to the proof of Theorem 2.1 in [6]. Suppose that  $n_t = n$ , and  
295 consider the events

$$\begin{aligned}E_{t,1} &\triangleq \left\{ V_t(n_*) - f\left(\frac{\alpha \ln(t)}{\gamma(n_*)-1}\right) \geq \sigma_*^2 S(\mathbf{w}) \right\}, \\ E_{t,2} &\triangleq \left\{ V_t(n) < \sigma_n^2 S(\mathbf{w}) - f\left(\frac{\alpha \ln(t)}{\gamma(n)-1}\right) \right\}, \\ E_{t,3} &\triangleq \left\{ \gamma(n) < 1 + \frac{\alpha \ln(T)}{\phi(\Delta_n S(\mathbf{w})/2)} \right\}.\end{aligned}$$

296 We claim that  $E_{t,1} \cup E_{t,2} \cup E_{t,3}$  must occur. Assume, by contradiction, that  $E_{t,i}$  are all false. We obtain

$$\begin{aligned} V_t(n_*) - f\left(\frac{\alpha \ln(t)}{\gamma_t(n_*) - 1}\right) &< \sigma_*^2 S(\mathbf{w}) = \sigma_n^2 S(\mathbf{w}) - \Delta_n S(\mathbf{w}) \\ &\leq V_t(n) + f\left(\frac{\alpha \ln(t)}{\gamma_t(n) - 1}\right) - \Delta_n S(\mathbf{w}). \end{aligned} \quad (\text{D.2})$$

297 By assumption  $E_{t,3}$  is false, and we have  $\gamma_t(n) - 1 \geq \alpha \ln(T)/\phi(\Delta_n S(\mathbf{w})/2)$ , which is equivalent to

$$\Delta_n S(\mathbf{w}) \geq 2f\left(\frac{\alpha \ln(T)}{\gamma_t(n) - 1}\right), \quad (\text{D.3})$$

298 If we use (D.3) in (D.2), then we obtain the following result, which contradicts the rule in (4):

$$V_t(n_*) - f\left(\frac{\alpha \ln(t)}{\gamma_t(n_*) - 1}\right) < V_t(n) - f\left(\frac{\alpha \ln(t)}{\gamma_t(n) - 1}\right).$$

299 For all  $n$  such that  $\Delta_n > 0$ , we define

$$M_n \triangleq \left\lceil \frac{\alpha \ln(T)}{\phi(\Delta_n S(\mathbf{w})/2)} \right\rceil.$$

300 We next upper bound  $\mathbb{E}_{\mathbf{w}}[\gamma_T(n)]$  as

$$\begin{aligned} \mathbb{E}_{\mathbf{w}}[\gamma_T(n)] &= \mathbb{E}_{\mathbf{w}}\left[\sum_{t=1}^T \mathbb{1}\{n_t = n \text{ and } \gamma_t(n) < M_n\}\right] + \mathbb{E}_{\mathbf{w}}\left[\sum_{t=1}^T \mathbb{1}\{n_t = n \text{ and } \gamma_t(n) \geq M_n\}\right] \\ &\leq M_n + \mathbb{E}_{\mathbf{w}}\left[\sum_{t=M_n+1}^T \mathbb{1}\{n_t = n \text{ and } \gamma_t(n) \geq M_n\}\right]. \end{aligned} \quad (\text{D.4})$$

301 In (D.4), we observe that  $\gamma_t(n) \geq M_n$  is equivalent to  $E_{t,3}$  being false, which is further equivalent to  
302  $E_{t,1} \cup E_{t,2}$  being true, i.e.,  $E_{t,1}$  or  $E_{t,2}$  must occur. Therefore we can further upper bound (D.4) as

$$\begin{aligned} \mathbb{E}_{\mathbf{w}}[\gamma_T(n)] &\leq M_n + \mathbb{E}_{\mathbf{w}}\left[\sum_{t=M_n+1}^T \mathbb{1}\{E_{t,1} \text{ or } E_{t,2} \text{ is true}\}\right] \\ &= M_n + \sum_{t=M_n+1}^T \Pr(E_{t,1} \cup E_{t,2} \text{ is true}) \\ &\leq M_n + \sum_{t=M_n+1}^T \Pr(E_{t,1}) + \sum_{t=M_n+1}^T \Pr(E_{t,2}). \end{aligned} \quad (\text{D.5})$$

303 where we used the union bound. We upper bound  $\Pr(E_{t,1})$  for each  $t = M_n + 1, \dots, T$ . Note that

$$\Pr(E_{t,1} = 1) = \Pr\left(V_t(n_*) - f\left(\frac{\alpha \ln(t)}{\gamma_t(n_*) - 1}\right) \geq \sigma_*^2 S(\mathbf{w})\right), \quad (\text{D.6})$$

304 where  $\gamma_t(n_*)$  can take values in  $\{2, \dots, t\}$ . Hence we apply the union bound in (D.6), which yields

$$\Pr(E_{t,1} = 1) \leq \sum_{s=1}^t \Pr\left(V'_s(n_*) - f\left(\frac{\alpha \ln(t)}{s}\right) \geq \sigma_*^2 S(\mathbf{w})\right) \leq \sum_{s=1}^t \frac{1}{t^\alpha} = t^{1-\alpha}, \quad (\text{D.7})$$

305 where (D.7) follows from (13). Here,  $V'_s(n_*)$  is the trace of a sample covariance matrix given  $s+2$   
306 independent random vectors with sub-Gaussian components with the parameter  $\sigma_*^2 S(\mathbf{w})$ . Hence we  
307 obtain

$$\sum_{t=M_n+1}^T \Pr(E_{t,1} = 1) \leq \sum_{t=M_n+1}^T t^{1-\alpha} \leq \sum_{t=1}^{\infty} t^{1-\alpha} \leq 1 + \int_1^{\infty} t^{1-\alpha} dt = \frac{\alpha-1}{\alpha-2}. \quad (\text{D.8})$$

308 The same upper bound holds for  $\Pr(E_{t,2} = 1)$  so that

$$\sum_{t=M_n+1}^T \Pr(E_{t,2} = 1) \leq \frac{\alpha-1}{\alpha-2}.$$

309 By incorporating these upper bounds into (D.5) we obtain

$$\mathbb{E}_{\mathbf{w}}[\gamma(n)] \leq M_n + 2(\alpha - 1)/(\alpha - 2).$$

310 Finally we use this result to get

$$\mathbb{E}_{\mathbf{w}} \left[ \sum_{n=1}^N \Delta_n \gamma_T(n) \right] S(\mathbf{w}) \leq (C_1(\mathbf{w}) \ln(T) + C_2) S(\mathbf{w}),$$

311 where  $C_1(\mathbf{w})$  and  $C_2$  are defined in (D.1). □
